# Supplementary material for: Learning Restricted Regular Expressions with Interleaving
Source: arXiv:1904.13164 source file (2019-04-30)
Supplement: Supplementary file 1 [file paper_appendix.tex]

\section*{Appendix}
\begin{table*}[h]

\caption{The List of Abbreviations for Words in \textbf{NASA}}
\center
\begin{tabular}{|c|c||c|c||c|c||c|c||c|c|}
\hline
\textbf{Word}& \textbf{Abbr.} &\textbf{Word}& \textbf{Abbr.}& \textbf{Word}& \textbf{Abbr.}&\textbf{Word}& \textbf{Abbr.}&\textbf{Word}& \textbf{Abbr.}  \\

\hline
title& $a_{1}$ &altname&  $a_{2}$& reference&  $a_{3}$&keywords&  $a_{4}$&descriptions&  $a_{5}$  \\
\hline
tableHead& $a_{6}$ &fitsFile&  $a_{7}$& history&  $a_{8}$&identifier&  $a_{9}$&textFile&  $a_{10}$  \\
\hline
\end{tabular}

\end{table*}

\begin{table*}[h]

\caption{The List of Abbreviations for Words in \textbf{DBLP}}
\center
\begin{tabular}{|c|c||c|c||c|c||c|c|}
\hline
\textbf{Word}& \textbf{Abbr.} &\textbf{Word}& \textbf{Abbr.}& \textbf{Word}& \textbf{Abbr.}&\textbf{Word}& \textbf{Abbr.}  \\

\hline
editor& $a_{1}$ &ee&  $a_{7}$& publisher&  $a_{13}$&isbn&  $a_{19}$  \\

\hline
author& $a_{2}$ &journal& $a_{8}$& title&  $a_{14}$&series&  $a_{20}$  \\

\hline
booktitle& $a_{3}$ &month& $a_{9}$&url&  $a_{15}$&school&  $a_{21}$  \\

\hline
cdrom& $a_{4}$ &note&$a_{10}$& volume& $a_{16}$&chapter& $a_{22}$  \\

\hline
cite& $a_{5}$ &number& $a_{11}$& year& $a_{17}$&publnr&  $a_{23}$  \\

\hline
crossref& $a_{6}$ &pages&$a_{12}$&address&  $a_{18}$&&    \\

\hline
\end{tabular}
\label{abb1}
\end{table*}

\begin{table*}[h]

\caption{The List of Abbreviations for Words in \textbf{table(DocBook)}}
\center
\begin{tabular}{|c|c||c|c||c|c||c|c|}

\hline
\textbf{Word}& \textbf{Abbr.} &\textbf{Word}& \textbf{Abbr.}& \textbf{Word}& \textbf{Abbr.}&\textbf{Word}& \textbf{Abbr.} \\

\hline
attlist& $a_{1}$ &info&  $a_{2}$& alt&  $a_{3}$&inlines&$a_{4}$\\
\hline
textobject& $a_{5}$ &mediaobject&  $a_{6}$& tgroup&  $a_{7}$&caption &$a_{8}$ \\
\hline
\end{tabular}

\end{table*}
